# Supplementary material for: Anomalous thermal broadening in the Shastry-Sutherland model and SrCu$_2($BO$_3)_2$
Source: arXiv:2405.18475 ancillary file (2024-05-28)
Supplement: Supplementary file 1 [file supplementary_material.pdf]

**Supplementary Material for “Anomalous thermal broadening in the  
Shastry-Sutherland model and  $\text{SrCu}_2(\text{BO}_3)_2$ ”**

(Dated: May 28, 2024)

## Abstract

In this supplementary section, we provide details of the thermal broadening calculation from perturbation theory.

### CONTENTS

|                                              |    |
|----------------------------------------------|----|
| Thermal broadening calculation outline       | 2  |
| Bond wave theory and lattice conventions     | 4  |
| $J/J_D$ perturbation theory and bound states | 5  |
| Single triplon states                        | 5  |
| Two triplon states                           | 7  |
| Susceptibility contributions                 | 12 |
| Further remarks on single triplon broadening | 16 |
| References                                   | 17 |

### THERMAL BROADENING CALCULATION OUTLINE

In this supplementary section we carry out a calculation of the dynamical structure factor for the Shastry-Sutherland model

$$S^{\alpha\beta}(\mathbf{q}, \omega) = -\frac{1}{\pi} \frac{1}{1 - e^{-\beta\omega}} \text{Im} [\chi^{\alpha\beta}(\mathbf{q}, \omega)] , \quad (1)$$

where  $\chi^{\alpha\beta}(\mathbf{q}, \omega)$  is the momentum and energy dependent susceptibility and  $\alpha, \beta$  are spin components. As the model is isotropic in spin space, without loss of generality we compute the  $zz$  component. This is given by

$$\chi^{zz}(\mathbf{q}, \omega) = - \int_0^\beta d\tau e^{i\omega_n \tau} \frac{1}{4N} \sum_{\mathbf{I}, \mathbf{J}} e^{-i\mathbf{q} \cdot (\mathbf{I} - \mathbf{J})} \langle S_{\mathbf{I}}^z(\tau) S_{\mathbf{J}}^z(0) \rangle \Big|_{\omega_n \rightarrow \eta - i\omega} . \quad (2)$$

Here  $N$  is the number of primitive lattice cells and the sum runs over all spins indexed by primitive cell, dimer  $\mathbf{d}$  and spin  $s$  e.g.  $\mathbf{I} = \mathbf{R}_I + \mathbf{d} + s(\mathbf{d})$ .

The correlator  $C(\mathbf{x} \equiv \mathbf{I} - \mathbf{J}, \tau) \equiv \langle S_{\mathbf{I}}^z(\tau) S_{\mathbf{J}}^z(0) \rangle$  can be written as

$$C(\mathbf{x}, \tau) = \frac{1}{Z} \sum_{m,n} e^{-\beta E_m} \langle m | S_{\mathbf{I}}^z(\tau) | n \rangle \langle n | S_{\mathbf{J}}^z(0) | m \rangle, \quad (3)$$

where states labeled by  $m$  and  $n$  run over the exact eigenstates of the system.

We then separate the states into sets  $\Gamma_r, \Gamma_s$  defined by the triplon number  $r, s$ . Using

$$\langle \Gamma_r | S_{\mathbf{I}}^z(\tau) | \Gamma_s \rangle = e^{-\tau(E_{\Gamma_s} - E_{\Gamma_r})} \langle \Gamma_r | S_{\mathbf{I}}^z | \Gamma_s \rangle \quad (4)$$

and carrying out the imaginary time integration we find:

$$\chi^{zz}(\mathbf{q}, \omega) = \frac{1}{4N} \frac{1}{Z} \sum_{\Gamma_r, \Gamma_s} \sum_{\mathbf{I}, \mathbf{J}} e^{-i\mathbf{q} \cdot (\mathbf{I} - \mathbf{J})} \langle \Gamma_r | S_{\mathbf{I}}^z | \Gamma_s \rangle \langle \Gamma_s | S_{\mathbf{J}}^z | \Gamma_r \rangle \left( \frac{e^{-\beta E_{\Gamma_r}} - e^{-\beta E_{\Gamma_s}}}{\omega + i\eta + E_{\Gamma_r} - E_{\Gamma_s}} \right). \quad (5)$$

The strategy we adopt for computing the thermal broadening of the dynamical structure factor originates from Refs. [1, 2] which contain calculations of thermal broadening in spin chains and, in particular, a demonstration of asymmetric lineshape broadening in the models considered (alternative variants exist, see, e.g., Refs. [3, 4]). The first simplification we make is to focus on temperatures smaller than the single triplon gap  $\Delta$ . Since higher energy excitations are suppressed by the Boltzmann weight we concentrate only on contributions to the susceptibility coming from few triplon excitations. In particular, we write

$$\chi^{zz}(\mathbf{q}, \omega) = \frac{1}{Z} \sum_{r,s=0}^{\infty} C_{rs} \approx \frac{1}{Z} (C_{10} + C_{01} + C_{11} + C_{12} + C_{21}) \quad (6)$$

where the sum is over all  $r, s$  triplon contributions.

We use notation  $D(\mathbf{q}, \omega)$  for the single triplon propagator which is simply

$$(1 - e^{-\beta\Delta}) D(\mathbf{q}, \omega) = C_{10} + C_{01} \quad (7)$$

with

$$D(\mathbf{q}, \omega) = \frac{1}{8} \left[ 2 - \cos\left(\frac{q_x + q_y}{2}\right) - \cos\left(\frac{q_x - q_y}{2}\right) \right] \left( \frac{1}{\omega + i\eta - \Delta} - \frac{1}{\omega + i\eta + \Delta} \right). \quad (8)$$

Now we suppose that interactions between the triplons are folded into a self-energy  $\Sigma(\mathbf{q}, \omega)$  appearing in a Dyson expansion for the susceptibility component

$$\chi^{zz}(\mathbf{q}, \omega) = \frac{D(\mathbf{q}, \omega)}{1 - D(\mathbf{q}, \omega) \Sigma(\mathbf{q}, \omega)} \approx D(\mathbf{q}, \omega) (1 + D(\mathbf{q}, \omega) \Sigma(\mathbf{q}, \omega)). \quad (9)$$

Matching Eqs. (6) and (9) leads to a resummed expression for the self-energy

$$\Sigma(\mathbf{q}, \omega) = D^{-2} (C_{11} + C_{12} + C_{21} - e^{-\beta\epsilon} D - Z_1(1 - e^{-\beta\epsilon})D) \quad (10)$$

where the partition sum has been split into contributions labeled by triplon number  $Z = 1 + Z_1 + Z_2 + \dots$  and where we have neglected  $Z_2$  and higher terms as they are suppressed exponentially at low temperatures.

## BOND WAVE THEORY AND LATTICE CONVENTIONS

The Shastry-Sutherland model is a spin one-half localized spin model on a two dimensional lattice with a square primitive cell  $\mathbf{R}_1 = (1, 0)$  and  $\mathbf{R}_2 = (0, 1)$ ,  $\mathbf{R}_I = m_I \mathbf{R}_1 + n_I \mathbf{R}_2$ , and a four sublattice basis:

$$\mathbf{r}_{A1} = (0, 0), \quad \mathbf{r}_{A2} = \left(\frac{1}{2}, \frac{1}{2}\right), \quad \mathbf{r}_{B1} = \left(1, \frac{1}{2}\right), \quad \mathbf{r}_{B2} = \left(\frac{1}{2}, 1\right). \quad (11)$$

For site  $i$ , we shall find it helpful to separate out the dimer center  $\mathbf{d}_i$  with  $i = A, B$

$$\mathbf{d}_A = \left(\frac{1}{4}, \frac{1}{4}\right), \quad \mathbf{d}_B = \left(\frac{3}{4}, \frac{3}{4}\right) \quad (12)$$

and the spin relative to the dimer center  $\mathbf{s}_i$  where, implicitly, the latter depends on the index  $A$  or  $B$  of the sublattice

$$\mathbf{s}_{A1} = \left(-\frac{1}{4}, -\frac{1}{4}\right), \quad \mathbf{s}_{A2} = \left(\frac{1}{4}, \frac{1}{4}\right), \quad \mathbf{s}_{B1} = \left(\frac{1}{4}, -\frac{1}{4}\right), \quad \mathbf{s}_{B2} = \left(-\frac{1}{4}, +\frac{1}{4}\right). \quad (13)$$

The magnetic interactions consist of nearest-neighbor and next-nearest-neighbor Heisenberg exchange

$$H = J_D \sum_{\langle i, j \rangle} \mathbf{S}_i \cdot \mathbf{S}_j + J \sum_{\langle\langle i, j \rangle\rangle} \mathbf{S}_i \cdot \mathbf{S}_j. \quad (14)$$

The ground state of the model for  $J/J_D \lesssim 0.65$  is a dimer covering with singlets on sites  $A1 - A2$  and  $B1 - B2$  which are coupled by  $J_D$ . This breaks no symmetries and there is a crossover as the temperature is lowered.

It is convenient to work with a bond wave representation of the ground state and magnetic excitations due to Sachdev and Bhatt [5]. The starting point is to introduce operators that create singlet and triplet states from the vacuum. In the Shastry-Sutherland model these operators are

defined on all dimers.

$$|s\rangle = s^\dagger |\text{VAC}\rangle = \frac{1}{\sqrt{2}} (|\uparrow\downarrow\rangle - |\downarrow\uparrow\rangle), \quad (15a)$$

$$|t_x\rangle = t_x^\dagger |\text{VAC}\rangle = -\frac{1}{\sqrt{2}} (|\uparrow\uparrow\rangle - |\downarrow\downarrow\rangle), \quad (15b)$$

$$|t_y\rangle = t_y^\dagger |\text{VAC}\rangle = \frac{i}{\sqrt{2}} (|\uparrow\uparrow\rangle + |\downarrow\downarrow\rangle), \quad (15c)$$

$$|t_z\rangle = t_z^\dagger |\text{VAC}\rangle = \frac{1}{\sqrt{2}} (|\uparrow\downarrow\rangle + |\downarrow\uparrow\rangle). \quad (15d)$$

These must satisfy the constraint

$$s^\dagger s + \sum_{\alpha} t_{\alpha}^\dagger t_{\alpha} = 1. \quad (16)$$

In terms of the singlet and triplet operators, the spin one-half operators are

$$S_1^\alpha = \frac{1}{2} \left( s^\dagger t_{\alpha} + t_{\alpha}^\dagger s - i\epsilon_{\alpha\beta\gamma} t_{\beta}^\dagger t_{\gamma} \right), \quad (17a)$$

$$S_2^\alpha = \frac{1}{2} \left( -s^\dagger t_{\alpha} - t_{\alpha}^\dagger s - i\epsilon_{\alpha\beta\gamma} t_{\beta}^\dagger t_{\gamma} \right). \quad (17b)$$

The intra-dimer exchange coupling  $\mathbf{S}_1 \cdot \mathbf{S}_2$  can be written in terms of the bond operators as follows:

$$-\frac{3}{4} s^\dagger s + \frac{1}{4} \sum_{\alpha=x,y,z} t_{\alpha}^\dagger t_{\alpha}, \quad (18)$$

after imposing the constraint.

An example of an exchange coupling between neighboring dimers is

$$\frac{1}{2} i\epsilon_{\alpha\beta\gamma} t_{i\beta}^\dagger t_{i\gamma} \left( s_j^\dagger t_{j\alpha} + t_{j\alpha}^\dagger s_j - i\epsilon_{\alpha\sigma\tau} t_{j\sigma}^\dagger t_{j\tau} \right), \quad (19)$$

where the triplon indices are in the Cartesian basis  $x, y, z$ .

Taken together Eqs. (18) and (19) reveal that, for sufficiently small  $J/J_D$ , the ground state is obtained by condensing singlets while the lowest energy excitations are triply degenerate “triplons” lying at energy  $J_D$ . As the coupling between singlets has no quadratic terms at this bare level the triplons are completely localized or, in momentum space, there are flat bands at energy  $J_D$  (to leading order in  $J/J_D$ ).

## $J/J_D$ PERTURBATION THEORY AND BOUND STATES

Now we consider the effects of carrying out perturbation theory in  $J/J_D$  within the dimer phase. In the material,  $\text{SrCu}_2(\text{BO}_3)_2$ ,  $J/J_D \approx 0.6$  and therefore not obviously in the perturbative regime

in the inter-dimer hopping. It turns out that physics in the Shastry-Sutherland model is remarkably localized especially in the ground state but also within the single triplon sector. In essence this localization, which originates from geometrical frustration of the Heisenberg coupling on this lattice, makes the perturbative treatment meaningful for much larger inter-dimer couplings than one might naively expect. This section essentially reviews results in Refs. [6–10]. We also refer the reader to a review [11] for a broader context.

### Single triplon states

As we have seen, the bare Hamiltonian to quadratic order has perfectly localized triplons. The single triplon gap is renormalized downwards by triplon interactions with the leading order contribution appearing already at  $O((J/J_D)^2)$ . To 4th order in  $J/J_D$  one finds:

$$\Delta = J_D \left( 1 - \left( \frac{J}{J_D} \right)^2 - \frac{1}{2} \left( \frac{J}{J_D} \right)^3 - \frac{1}{8} \left( \frac{J}{J_D} \right)^4 \right). \quad (20)$$

This is in very good agreement with exact diagonalization results throughout the dimer phase (see Fig. 4 in the main text).

Interaction effects also introduce a dispersion for the triplons. Eq. (19) contains cubic terms in the triplon operators of the schematic form  $t_i^\dagger t_i (t_j + t_j^\dagger)$  that effect a creation or annihilation of a triplon in the presence of a neighboring triplon. One can show that this term introduces an effective direct hopping term for the triplons to sixth order in perturbation theory [11–13]. The material  $\text{SrCu}_2(\text{BO}_3)_2$ , that is reasonably well described by the Shastry-Sutherland model in the dimer phase, has  $J/J_D \approx 0.6$  placing it close to the phase boundary of the dimer phase. For this value of  $J/J_D$  the single triplon dispersion is around 5% of the triplon gap so the bands remain quite flat [12]. Fig. 1 shows data from 28 site exact diagonalization recording the single triplon bandwidth as a function of  $J/J_D$ . The sixth order leading contribution to the bandwidth is evident from the figure with departures evident at larger coupling.

An important contribution to the triplon dispersion in the material comes from a Dzyaloshinsky-Moriya interaction (DMI). The magnitude of the DMI is roughly 5% of  $J_D$  [11, 14] and a direct fit of experimental data has been performed in Ref. [15]. The effects of DMI are particularly evident as they break the degeneracy of the triplon modes. As we shall see, the bound state modes in a given sector disperse on the scale of  $J^2$  but there is a splitting between sectors on the scale of  $J$ . Therefore the overall bandwidth of low-lying triplon states is dominated by the bound states

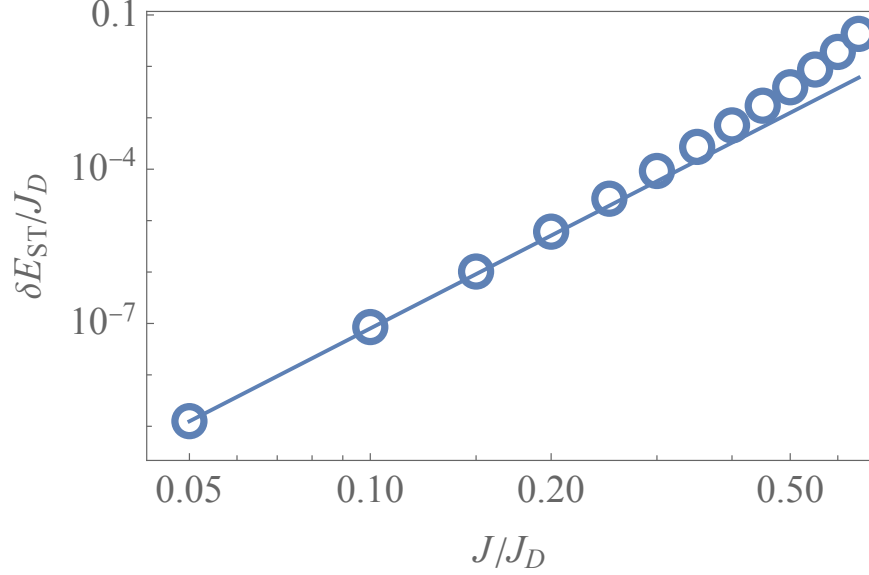

FIG. 1. Difference between maximum and minimum single triplon energies from  $N = 28$  exact diagonalization as a function of  $J/J_D$  and on a log-log scale (open circles). The straight line passing through the small  $J/J_D$  points is  $\delta E_{ST} \sim (J/J_D)^6$ .

and not by the presence of DMI. So while DMI certainly contributes to thermal broadening of the modes in the material (see also Section ), the principal effect is captured already in the pure Shastry-Sutherland model. Therefore we neglect the effects coming from DMI in the material.

### Two triplon states

As remarked on above, the exact dispersion relation of the single triplon states has a bandwidth that is much smaller than the triplon gap. This directly implies that the two triplon continuum is very narrow. Overall, geometrical frustration makes itself felt through the exact dimer ground state and through the presence of nearly localized triplon modes. The first place where the bare interactions generate physics almost on the scale of those interactions is through bound states of two triplons. It turns out that these are split on the scale of  $J$  and disperse on the scale of  $J^2$ .

To third order in  $J/J_D$  the bound and anti-bound states are composed of eight distinct triplon configurations up to lattice translations [10, 11]. These are shown in Fig. 2. For example, the states labeled (a) and (b) in sector I are connected by two correlated hopping processes generated from the cubic terms in perturbation theory where one process creates a triplon on the left which then annihilates a triplon at the top. The configurations shown participate for each of the bound

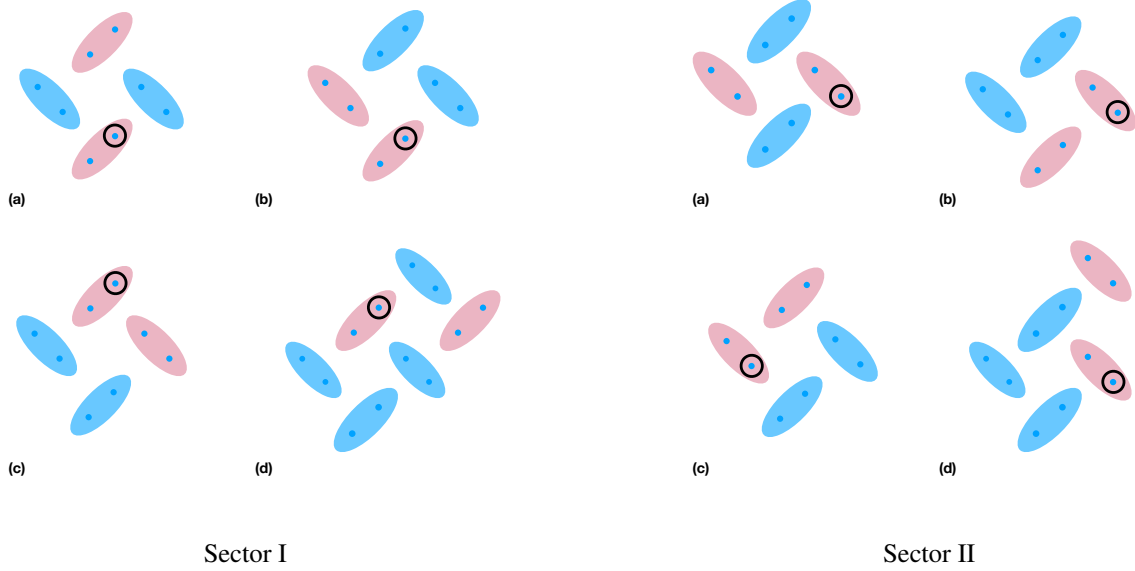

FIG. 2. Two triplon bound states connected to order  $(J'/J)^3$ . Sectors I and II are distinct at least up to third order.

state angular momentum sectors  $S = 0, 1, 2$ . The two sectors I and II are not connected to third order in perturbation theory. They are connected at higher order where also more configurations must be included.

The general form of an effective tight-binding model for Sector I is

$$H_I(\mathbf{q}) = \begin{pmatrix} 2\Delta + V_{\text{NNN}} & J_{\text{NN}} & J_{\text{NN}}e^{iq_y} & 0 \\ J_{\text{NN}} & 2\Delta + V_{\text{NN}} & J_3 & -J_{\text{NN}}e^{iq_x} \\ J_{\text{NN}}e^{-iq_y} & J_3 & 2\Delta + V_{\text{NN}} & -J_{\text{NN}} \\ 0 & -J_{\text{NN}}e^{-iq_x} & -J_{\text{NN}} & 2\Delta + V_{\text{NNN}} \end{pmatrix} \quad (21)$$

where aside from the gap  $\Delta$  in Eq. (20), the entries in the matrix depend on  $S$ . In particular, one finds for  $S = 2$ :

$$V_{\text{NN}} = \frac{J}{2} + \frac{J^2}{2J_D} - \frac{J^3}{8J_D^2} \quad (22)$$

$$V_{\text{NNN}} = \frac{J^3}{4J_D^2} \quad (23)$$

$$J_{\text{NN}} = \frac{J^2}{4J_D} + \frac{5J^3}{16J_D^2} \quad (24)$$

$$J_3 = \frac{J^2}{4J_D} + \frac{3J^3}{8J_D^2} \quad (25)$$

for  $S = 1$ :

$$V_{\text{NN}} = -\frac{J}{2} + \frac{J^2}{J_D} + \frac{7J^3}{8J_D^2} \quad (26)$$

$$V_{\text{NNN}} = -\frac{J^3}{4J_D^2} \quad (27)$$

$$J_{\text{NN}} = -\frac{J^2}{4J_D} - \frac{3J^3}{16J_D^2} \quad (28)$$

$$J_3 = \frac{J^2}{4J_D} + \frac{J^3}{8J_D^2} \quad (29)$$

and for  $S = 0$ :

$$V_{\text{NN}} = -J + \frac{J^2}{2J_D} + \frac{J^3}{J_D^2} \quad (30)$$

$$V_{\text{NNN}} = -\frac{J^3}{2J_D^2} \quad (31)$$

$$J_{\text{NN}} = -\frac{J^2}{2J_D} - \frac{J^3}{4J_D^2} \quad (32)$$

$$J_3 = -\frac{J^2}{2J_D}. \quad (33)$$

These results reveal that components (b) and (c) are bound to leading order in  $J$  with splitting  $+J/2$ ,  $-J/2$  and  $-J$  respectively for  $S = 2, 1, 0$ . Dispersion appears to order  $J^2$ . Sector II Hamiltonians are obtained by taking  $A \leftrightarrow B$  and  $q_x \rightarrow q_y$  and  $q_y \rightarrow -q_x$ .

The basis states for the bound states within each angular momentum sector take the form:

$$|\Phi_{0,0}\rangle = \Phi_{0,0}^\dagger |0\rangle = \frac{1}{\sqrt{3}} \left( t_1^\dagger t_{-1}^\dagger - t_0^\dagger t_0^\dagger + t_{-1}^\dagger t_1^\dagger \right) |0\rangle \quad (34)$$

$$|\Phi_{1,0}\rangle = \Phi_{1,0}^\dagger |0\rangle = \frac{1}{\sqrt{2}} \left( t_1^\dagger t_{-1}^\dagger - t_{-1}^\dagger t_1^\dagger \right) |0\rangle \quad (35)$$

$$|\Phi_{2,0}\rangle = \Phi_{2,0}^\dagger |0\rangle = \frac{1}{\sqrt{6}} \left( t_1^\dagger t_{-1}^\dagger + 2t_0^\dagger t_0^\dagger + t_{-1}^\dagger t_1^\dagger \right) |0\rangle \quad (36)$$

$$|\Phi_{1,1}\rangle = \Phi_{1,1}^\dagger |0\rangle = \frac{1}{\sqrt{2}} \left( t_1^\dagger t_0^\dagger - t_0^\dagger t_1^\dagger \right) |0\rangle \quad (37)$$

$$|\Phi_{1,-1}\rangle = \Phi_{1,-1}^\dagger |0\rangle = \frac{1}{\sqrt{2}} \left( t_0^\dagger t_{-1}^\dagger - t_{-1}^\dagger t_0^\dagger \right) |0\rangle \quad (38)$$

$$|\Phi_{2,1}\rangle = \Phi_{2,1}^\dagger |0\rangle = \frac{1}{\sqrt{2}} \left( t_1^\dagger t_0^\dagger + t_0^\dagger t_1^\dagger \right) |0\rangle \quad (39)$$

$$|\Phi_{2,-1}\rangle = \Phi_{2,-1}^\dagger |0\rangle = \frac{1}{\sqrt{2}} \left( t_0^\dagger t_{-1}^\dagger + t_{-1}^\dagger t_0^\dagger \right) |0\rangle \quad (40)$$

$$|\Phi_{2,2}\rangle = \Phi_{2,2}^\dagger |0\rangle = t_1^\dagger t_1^\dagger |0\rangle \quad (41)$$

$$|\Phi_{2,-2}\rangle = \Phi_{2,-2}^\dagger |0\rangle = t_{-1}^\dagger t_{-1}^\dagger |0\rangle. \quad (42)$$

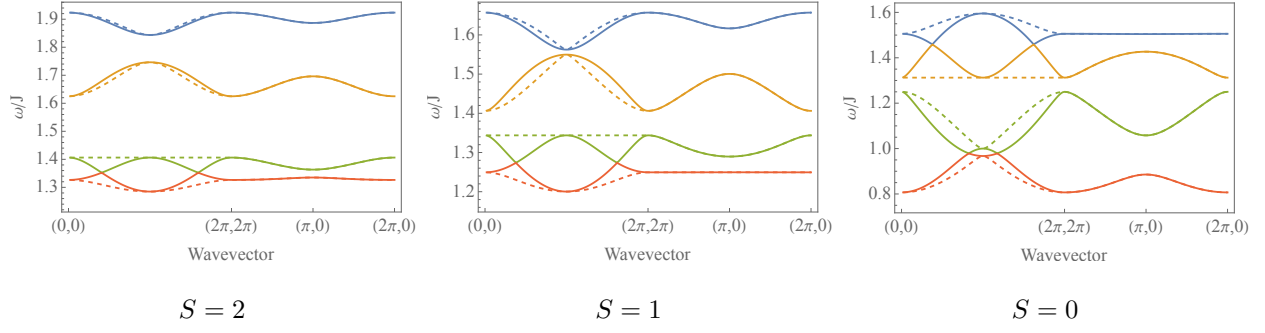

FIG. 3. Spectra of bound states to third order in perturbation theory in  $J/J_D = 0.5$ . From left to right these are for  $S = 2$ ,  $S = 1$  and  $S = 0$  angular momentum sectors. Solid lines are for Sector I and dashed lines for Sector II.

Using the configuration labels in real space in Fig. 2 we specify a notation for the two-triplon bound states. We label these configurations by  $\mu = a, b, c, d$  for the configuration and  $\sigma = I, II$  for the sector and refer each to the highlighted primitive cell position. We also need a label  $S, m$  for the angular momentum sector. In momentum space the states are

$$|\mathbf{P}, \mu, \sigma; S, m\rangle \equiv \frac{1}{\sqrt{N}} \sum_i \exp(i\mathbf{P} \cdot \mathbf{R}_i) |\mathbf{R}_i, \mu, \sigma; S, m\rangle. \quad (43)$$

The eigenstates are denoted  $|\mathbf{P}, M, \sigma; S, m\rangle$  where  $M$  runs over the four bands in each of the two sectors.

The two-triplon bound states,  $|\mathbf{P}, M, \sigma; S, m\rangle$  for eigenvalue  $M$ , obtained by diagonalizing the Hamiltonians given above, are

$$|\mathbf{P}, M, \sigma; S, m\rangle = \sum_{\mu=1}^4 v_{\mu}^M(\mathbf{P}, S, \sigma) |\mathbf{P}, \mu, \sigma; S, m\rangle. \quad (44)$$

The spectra of the two-triplon bound states to third order in perturbation theory in  $J/J_D$  are shown in Fig. 3. Each panel is for a different total angular momentum sector  $S = 2, 1, 0$  and each panel contains eight modes – four for each of sectors I and II defined above. Fig. 4 in the main text illustrates that the perturbative bound state band widths are in reasonable agreement with exact diagonalization results for  $J/J_D$  even as large as  $\sim 0.5$ . One notices from these figures that the lowest energy bound state mode lives in the singlet sector and that this crosses the single triplon energy at about  $J/J_D = 0.539$  (perturbation theory) and roughly  $J/J_D = 0.585$  (28 site ED). In  $\text{SrCu}_2(\text{BO}_3)_2$ , the exchange parameters are such that the lowest energy bound state mode is at about the single triplon energy.

| $\Gamma_{d'\sigma\mu}$ | $d'$                                                                                       |                                                                                              |
|------------------------|--------------------------------------------------------------------------------------------|----------------------------------------------------------------------------------------------|
|                        | A                                                                                          | B                                                                                            |
| Ia                     | $e^{i\mathbf{q}\cdot\hat{\mathbf{y}}} + e^{i(\mathbf{p}-\mathbf{q})\cdot\hat{\mathbf{y}}}$ | 0                                                                                            |
| Ib                     | $e^{-i(\mathbf{p}-\mathbf{q})\cdot\hat{\mathbf{x}}}$                                       | $e^{-i\mathbf{q}\cdot\hat{\mathbf{x}}}$                                                      |
| Ic                     | $e^{-i(\mathbf{p}-\mathbf{q})\cdot\hat{\mathbf{y}}}$                                       | $e^{-i\mathbf{q}\cdot\hat{\mathbf{y}}}$                                                      |
| Id                     | $e^{i\mathbf{q}\cdot\hat{\mathbf{x}}} + e^{i(\mathbf{p}-\mathbf{q})\cdot\hat{\mathbf{x}}}$ | 0                                                                                            |
| IIa                    | 0                                                                                          | $e^{-i\mathbf{q}\cdot\hat{\mathbf{x}}} + e^{-i(\mathbf{p}-\mathbf{q})\cdot\hat{\mathbf{x}}}$ |
| IIb                    | 1                                                                                          | 1                                                                                            |
| IIc                    | $e^{i\mathbf{q}\cdot(\hat{\mathbf{x}}+\hat{\mathbf{y}})}$                                  | $e^{i(\mathbf{p}-\mathbf{q})\cdot(\hat{\mathbf{x}}+\hat{\mathbf{y}})}$                       |
| IIId                   | 0                                                                                          | $e^{i\mathbf{q}\cdot\hat{\mathbf{y}}} + e^{i(\mathbf{p}-\mathbf{q})\cdot\hat{\mathbf{y}}}$   |

TABLE I. Matrix element contribution  $\Gamma_{d\sigma\mu}(\mathbf{p} - \mathbf{q}, \mathbf{q})$  defined in Eq. (46).

For the susceptibility contribution we require single triplon to bound state matrix elements:

$$\langle \mathbf{p}, \mu, \sigma; S, m | S_{ids}^z | \mathbf{q}, d', \tilde{m} \rangle \quad (45)$$

and we use the notation

$$\langle \mathbf{p}, \mu, \sigma; S, m | S_{ids}^z | \mathbf{q}, d', \tilde{m} \rangle \equiv \delta(d, d'; \sigma, \mu) \delta_{m, \tilde{m}} (1/N) (-)^{s+1} \alpha_{\tilde{m}}^{S, m} e^{-i(\mathbf{p}-\mathbf{q})\cdot\mathbf{R}_i} \Gamma_{d'\sigma\mu}(\mathbf{p} - \mathbf{q}, \mathbf{q}) \quad (46)$$

where  $\delta(d, d'; \sigma, \mu)$  enforces the constraints listed below on the dimer sublattices for a given configuration  $\mu$ . The  $\Gamma_{dd'\sigma\mu}(\mathbf{p} - \mathbf{q}, \mathbf{q})$  and  $\delta(d, d'; \sigma, \mu)$  are listed in the tables I and II, respectively.

The coefficients  $\alpha_{\tilde{m}}^{S, m}$  place constraints on the sum over the spin sectors and the resulting angular momentum degeneracies. In the susceptibilities they appear squared thus:

$$(\alpha_0^{0,0})^2 = \frac{1}{12} \quad (47)$$

$$(\alpha_0^{2,0})^2 = \frac{1}{6} \quad (48)$$

$$(\alpha_1^{1,1})^2 = \frac{1}{8} \quad (49)$$

$$(\alpha_{-1}^{1,-1})^2 = \frac{1}{8} \quad (50)$$

$$(\alpha_1^{2,1})^2 = \frac{1}{8} \quad (51)$$

$$(\alpha_{-1}^{2,-1})^2 = \frac{1}{8}. \quad (52)$$

Evidently  $\tilde{m} = m$  because  $S^z$  preserves a  $U(1)$  while breaking overall spin rotation symmetry.

| $\delta(d, d'; \sigma, \mu)$ | $d'$          |               |
|------------------------------|---------------|---------------|
|                              | A             | B             |
| Ia                           | $\delta_{dA}$ | —             |
| Ib                           | $\delta_{dB}$ | $\delta_{dA}$ |
| Ic                           | $\delta_{dB}$ | $\delta_{dA}$ |
| Id                           | $\delta_{dA}$ | —             |
| IIa                          | —             | $\delta_{dB}$ |
| IIb                          | $\delta_{dB}$ | $\delta_{dA}$ |
| IIc                          | $\delta_{dB}$ | $\delta_{dA}$ |
| IId                          | —             | $\delta_{dB}$ |

TABLE II. Matrix element contribution  $\delta(d, d'; \sigma, \mu)$  defined in Eq. (46).

## SUSCEPTIBILITY CONTRIBUTIONS

The contribution to the susceptibility arising from transitions from the ground state to the single triplon states is

$$\chi^{zz}(\mathbf{q}, \omega)|_{01/10;AA} = \frac{1}{Z} \frac{1}{8} (1 - e^{-\beta\Delta}) \left[ 1 - \cos\left(\frac{q_x + q_y}{2}\right) \right] \left( \frac{1}{\omega + i\eta - \Delta} - \frac{1}{\omega + i\eta + \Delta} \right) \quad (53)$$

$$\chi^{zz}(\mathbf{q}, \omega)|_{01/10;BB} = \frac{1}{Z} \frac{1}{8} (1 - e^{-\beta\Delta}) \left[ 1 - \cos\left(\frac{q_x - q_y}{2}\right) \right] \left( \frac{1}{\omega + i\eta - \Delta} - \frac{1}{\omega + i\eta + \Delta} \right) \quad (54)$$

for the A and B sublattice dimers. For convenience, we show again the form of the single particle propagator (Eq. (7)) that follows from these equations

$$D(\mathbf{q}, \omega) = \frac{1}{8} \left[ 2 - \cos\left(\frac{q_x + q_y}{2}\right) - \cos\left(\frac{q_x - q_y}{2}\right) \right] \left( \frac{1}{\omega + i\eta - \Delta} - \frac{1}{\omega + i\eta + \Delta} \right). \quad (55)$$

Here we have assumed that the triplons are dispersionless with energy  $\Delta$  (Eq. (20)). The dynamical structure factor computed from this susceptibility is delta peaked at the single triplon energy and only the coefficient of the delta function is temperature dependent. We note that only matrix elements connecting the ground state to the  $S^z = 0$  single triplon states contribute to the susceptibility.

For perfectly localized triplon modes, the matrix elements connecting single triplon to single triplon states vanish so that the contribution  $C_{11}$  in Eq. (10) for the self-energy is zero. As we have discussed, this ceases to be the case once high order perturbative processes are included that allow

for single triplon hopping. This can be expected to give the leading contribution to the direct broadening of the delta function peak at the single triplon energies. However, the resulting linewidth is bounded by the very narrow bandwidth of the triplon mode and therefore cannot account for the extent of the observed broad response in energy. In the following we work consistently with the flat triplon mode.

We now report the part of the susceptibility connecting the single triplon states with unbound two triplon states first of all without any restriction on the number of the latter states coming from the presence of bound states.

$$\chi^{zz}(\mathbf{q}, \omega)|_{12(\text{free});AA} = \frac{1}{8Z} \frac{3}{4} (4N+2) \left( \frac{e^{-\beta\Delta} - e^{-2\beta\Delta}}{\omega + i\eta - \Delta} \right) \left[ 1 - \cos\left(\frac{q_x + q_y}{2}\right) \right] \quad (56)$$

$$\chi^{zz}(\mathbf{q}, \omega)|_{12(\text{free});BB} = \frac{1}{8Z} \frac{3}{4} (4N+2) \left( \frac{e^{-\beta\Delta} - e^{-2\beta\Delta}}{\omega + i\eta - \Delta} \right) \left[ 1 - \cos\left(\frac{q_x - q_y}{2}\right) \right]. \quad (57)$$

We note that the pieces proportional to  $N$  are identical to the ground state to single triplon contribution to the susceptibility after multiplying by  $3Ne^{-\beta\Delta}D(\mathbf{q}, \omega)$  which is nothing other than  $(1 - e^{-\beta\Delta})Z_1D(\mathbf{q}, \omega)$  in Eq. (10) where  $Z_1$  is the single triplon contribution to the partition sum.

The susceptibility connecting single triplon to two free triplon states given above overcounts because some of the two free triplon states participate in bound states. In particular, inspection of the matrix element connecting single triplons to two free triplon states reveals that for fixed initial and final state momentum and with one primitive lattice position fixed by the spin whose matrix element is computed, there remains a sum over real space positions. Within this sum there are contributions coming from configurations illustrated in Fig. 2. In other words, the matrix element is corrected from  $M(\mathbf{p}_1, \mathbf{p}_2, \mathbf{p}, \mathbf{i})$  to  $M(\mathbf{p}_1, \mathbf{p}_2, \mathbf{p}, \mathbf{i}) - \delta M$  where the  $\delta M$  subtracts off the configurations that contribute to the bound states. Once these have been accounted for we find for the free triplon contribution

$$\begin{aligned} (C_{12} + C_{21})|_{\text{free}} &= (1 - e^{-\beta\Delta})Z_1D(\mathbf{q}, \omega) \\ &= -\frac{21}{16} (e^{-\beta\Delta} - e^{-2\beta\Delta}) F(q_x, q_y) \left( \frac{1}{\omega + i\eta - \Delta} - \frac{1}{\omega + i\eta + \Delta} \right) \end{aligned} \quad (58)$$

where

$$F(q_x, q_y) = \left[ 2 - \cos\left(\frac{q_x + q_y}{2}\right) - \cos\left(\frac{q_x - q_y}{2}\right) \right]. \quad (59)$$

Here we have accounted for the factor 2 coming from the sum over spins for a fixed dimer. This has  $1/\eta^2$  divergences like the single triplon propagator. Evidently, this term contributes only at the single triplon energy and is suppressed exponentially in the single triplon gap.

By considering the bound states of two triplons we find a response over a broad energy range. The contributions to Eq. (10) are

$$C_{12}|_{\text{bound}} = \frac{1}{4N} \sum_{\mathbf{k}, m, d, \sigma, \mu, \tilde{\mu}} \sum_{d_i, d_j, s_i, s_j} e^{-i\mathbf{q} \cdot (d_i - d_j + s_i - s_j)} (\alpha_m^{S, m})^2 (-)^{s_i + s_j} \delta(d_i, d; \sigma, \mu) \delta(d_j, d; \sigma, \tilde{\mu})$$

$$\Gamma_{d\sigma\tilde{\mu}}(\mathbf{q}, \mathbf{k} - \mathbf{q}) \Gamma_{d\sigma\mu}^*(\mathbf{q}, \mathbf{k} - \mathbf{q}) \left( \frac{e^{-\beta\Delta} - e^{-\beta E_{\mathbf{k}, M, S, \sigma}^{(2)}}}{\omega + i\eta + \Delta - E_{\mathbf{k}, M, S, \sigma}^{(2)}} \right) v_{\mu}^M(\mathbf{k}, S, \sigma) v_{\tilde{\mu}}^{*M}(\mathbf{k}, S, \sigma)$$
(60)

and

$$C_{21}|_{\text{bound}} = \frac{1}{4N} \sum_{\mathbf{k}, m, d, \sigma, \mu, \tilde{\mu}} \sum_{s_i, s_j} e^{-i\mathbf{q} \cdot (d_i - d_j + s_i - s_j)} (\alpha_m^{S, m})^2 (-)^{s_i + s_j} \delta(d_i, d; \sigma, \mu) \delta(d_j, d; \sigma, \tilde{\mu})$$

$$\Gamma_{d\sigma\mu}(-\mathbf{q}, \mathbf{k} + \mathbf{q}) \Gamma_{d\sigma\tilde{\mu}}^*(-\mathbf{q}, \mathbf{k} + \mathbf{q}) \left( \frac{e^{-\beta E_{\mathbf{k}, M, S, \sigma}^{(2)}} - e^{-\beta\Delta}}{\omega + i\eta + E_{\mathbf{k}, M, S, \sigma}^{(2)} - \Delta} \right) v_{\mu}^{*M}(\mathbf{k}, S, \sigma) v_{\tilde{\mu}}^M(\mathbf{k}, S, \sigma).$$
(61)

As noted above, in  $\text{SrCu}_2(\text{BO}_3)_2$  the minimum energy singlet two-triplon bound states coincide with the single triplon energy. Eq. (60) implies, then, that there is an inelastic response in the Shastry-Sutherland model at finite temperatures extending from very low energies. In particular, the lowest energy bound states live in the singlet sector  $S = 0$  for which the energies  $E_{\mathbf{k}, M, 0, \sigma}^{(2)}$  extend upwards from around  $\Delta$ . Therefore the condition  $\omega = E_{\mathbf{k}, M, S, \sigma}^{(2)} - \Delta$  (from the denominator in Eq. (60)) “clicks” at energies  $\omega$  much smaller than  $\Delta$ . This is the central observation accounting for the experimentally observed broad response in the material.

In the main text we present results from a direct evaluation of the dynamical structure factor (Eqs. (1) and (9)) including the expression Eq. (10) for the self-energy. The integration over momenta in the bound state contribution to  $C_{12}$  and  $C_{21}$  is performed numerically with fixed finite  $\eta$ . The number of integration points  $N$  is chosen to reach convergence with integration grid fine enough to be significantly smaller than the artificial width set by  $\eta$ . The width  $\eta$  itself is chosen to be  $0.004J_D$  so much smaller than the bandwidth of the bound states.

The results reveal a very broad temperature dependent inelastic response originating from the bound state modes that are low-lying in relation to the single triplon modes. The single triplon peak remains delta spiked in our calculation unlike the triplon mode in the alternating Heisenberg chain studied by James *et al.* [2]. The origin of the difference is the presence of  $1/\eta^4$  divergences at the single triplon energy in the one-to-two particle susceptibility in the one dimensional case that are

cured by computing the resummed self-energy. In the Shastry-Sutherland model, the divergences are much less severe. There are logarithmic divergences in the one-to-two particle susceptibility in the Shastry-Sutherland model in the bound state channel coming from van Hove singularities in the bound state band structure at various energies depending on  $J/J_D$  that are presumably resolved at higher order in the low temperature expansion. There is also a  $1/\eta^2$  divergence coming from one to two free triplon susceptibility that have the effect of reducing the spectral weight in the delta peak as a function of temperature.

Finally, we remark on the connection between the Shastry-Sutherland model and thermal broadening in other quantum magnets. As shown in the main text the magnitude and temperature dependence of the thermal broadening in  $\text{SrCu}_2(\text{BO}_3)_2$  are captured by dynamical METTS on the Shastry-Sutherland model. The low temperature expansion suggests that the origin of this anomalous broadening is the small gap between the single triplon modes and the bound states. An intuition for this effect is that when there is a small thermal population of triplons at low temperature, excitation of a second triplon spectroscopically can have weight in the singlet bound state sector at very low energies thus producing a broad response. The magnitude of this response is expected to increase with the ambient thermal population of triplons.

What sets the Shastry-Sutherland model apart from typical quantum magnets in this regard? The answer would seem to rely on the peculiar fine-tuning of  $\text{SrCu}_2(\text{BO}_3)_2$ . Other quantum magnets, for the purposes of this discussion, typically fall into two classes: gapped and (nearly) gapless. Gapless quantum magnets have single particle modes appearing, for the most part, among two particle states in the same energy range with broadening induced at zero temperature by matrix elements connecting these states. We would typically not expect thermal broadening to be especially dramatic in such gapless systems as there is (i) a broad continuum at low energies and (ii) zero temperature broadening. If, instead, the magnet is gapped on scale  $\Delta$ , it is typical for the two particle states to have minimum at  $2\Delta$ . This means that the thermal response is expected at  $\omega \sim \Delta$ . In contrast, in  $\text{SrCu}_2(\text{BO}_3)_2$ , it begins at low energies because the material is poised close to a phase boundary connected to the condensation of bound states so that states are available at anomalously low energies compared to the single particle gap.

## FURTHER REMARKS ON SINGLE TRIPLON BROADENING

In the previous section, we pointed out that, when working consistently to third order in  $J/J_D$  perturbation theory, the triplon modes are dispersionless and that the susceptibility coming from one triplon to one triplon processes,  $C_{11}$ , vanishes. The triplons in the Shastry-Sutherland model, however, do disperse albeit weakly. The, leading order, contribution to the hopping (at sixth order in  $J/J_D$ ) is between identical neighboring sublattices so the single triplon Hamiltonian remains diagonal in this basis. Even higher order processes break the six-fold degenerate triplons into a pair of three-fold degenerate modes. DMI is known to be an important component of the magnetic couplings in  $\text{SrCu}_2(\text{BO}_3)_2$  at roughly the 10% level and it leads directly to a hopping term for the triplons.

Here we compute the susceptibility  $C_{11}$  in the presence of triplon dispersion and estimate the importance of this contribution to the finite temperature response compared to the contributions coming from bound states of two triplons. In general the relevant contribution to the susceptibility is

$$\chi^{zz}(\mathbf{q}, \omega) = \frac{1}{4NZ} \sum_{m,m',d,d'} \sum_{\mathbf{p},\mathbf{k},\mathbf{I},\mathbf{J}} e^{-i\mathbf{q}\cdot(\mathbf{I}-\mathbf{J})} \langle \mathbf{p}dm | S_{\mathbf{I}}^z | \mathbf{k}d'm' \rangle \langle \mathbf{k}d'm' | S_{\mathbf{J}}^z | \mathbf{p}dm \rangle \left( \frac{e^{-\beta E_{\mathbf{p}}} - e^{-\beta E_{\mathbf{k}}}}{\omega + i\eta + E_{\mathbf{p}} - E_{\mathbf{k}}} \right) \quad (62)$$

where  $E_{\mathbf{p}}$  is the single triplon energy at momentum  $\mathbf{p}$ .

If the hopping matrix element is diagonal in the sublattice basis then we obtain

$$C_{11}(\mathbf{q}, \omega) = \frac{1}{2N} \sum_{\mathbf{k}} \left( 1 + \cos\left(\frac{q_x}{2}\right) \cos\left(\frac{q_y}{2}\right) \right) \left( \frac{e^{-\beta E_{\mathbf{k}-\mathbf{q}}} - e^{-\beta E_{\mathbf{k}}}}{\omega + i\eta + E_{\mathbf{k}-\mathbf{q}} - E_{\mathbf{k}}} \right). \quad (63)$$

Evidently, if the triplon bandwidth goes to zero, this contribution vanishes as previously claimed.

The details of the  $C_{11}$  contribution to the dynamical response function depends on the nature of the dispersion relation and the magnetic couplings. However, Eq. (63) can be expected to capture the general dependence on energy  $\omega$ . For single triplon modes with bandwidth  $2g \ll \Delta$ ,  $C_{11}$  will have its principal effect at low energies extending up to  $\omega = 4g$ . To put this in perspective the bandwidth in  $\text{SrCu}_2(\text{BO}_3)_2$  is about 10% of the 3 meV gap so one should expect the single triplon dispersion to contribute up to an energy of about 0.6 meV independent of the nature of the matrix elements. DMI will tend to introduce some small direct broadening of the single triplon peak but this is expected to be much smaller than the broad contribution originating from the bound states as the imaginary part of the self-energy is suppressed at higher energies than  $4g$ .

- 
- [1] F. H. L. Essler and R. M. Konik, Finite-temperature lineshapes in gapped quantum spin chains, [Phys. Rev. B \*\*78\*\*, 100403 \(2008\)](#).
  - [2] A. J. A. James, F. H. L. Essler, and R. M. Konik, Finite-temperature dynamical structure factor of alternating Heisenberg chains, [Phys. Rev. B \*\*78\*\*, 094411 \(2008\)](#).
  - [3] E. S. Klyushina, A. C. Tiegell, B. Fauseweh, A. T. M. N. Islam, J. T. Park, B. Klemke, A. Honecker, G. S. Uhrig, S. R. Manmana, and B. Lake, Magnetic excitations in the  $S = \frac{1}{2}$  antiferromagnetic-ferromagnetic chain compound  $\text{BaCu}_2\text{V}_2\text{O}_8$  at zero and finite temperature, [Phys. Rev. B \*\*93\*\*, 241109 \(2016\)](#).
  - [4] B. Fauseweh, F. Groitl, T. Keller, K. Rolfs, D. A. Tennant, K. Habicht, and G. S. Uhrig, Time-dependent correlations in quantum magnets at finite temperature, [Phys. Rev. B \*\*94\*\*, 180404 \(2016\)](#).
  - [5] S. Sachdev and R. N. Bhatt, Bond-operator representation of quantum spins: Mean-field theory of frustrated quantum Heisenberg antiferromagnets, [Phys. Rev. B \*\*41\*\*, 9323 \(1990\)](#).
  - [6] P. Lemmens, M. Grove, M. Fischer, G. Güntherodt, V. N. Kotov, H. Kageyama, K. Onizuka, and Y. Ueda, Collective Singlet Excitations and Evolution of Raman Spectral Weights in the 2D Spin Dimer Compound  $\text{SrCu}_2(\text{BO}_3)_2$ , [Phys. Rev. Lett. \*\*85\*\*, 2605 \(2000\)](#).
  - [7] S. Miyahara and K. Ueda, Exact Dimer Ground State of the Two Dimensional Heisenberg Spin System  $\text{SrCu}_2(\text{BO}_3)_2$ , [Phys. Rev. Lett. \*\*82\*\*, 3701 \(1999\)](#).
  - [8] K. Totsuka, S. Miyahara, and K. Ueda, Low-Lying Magnetic Excitation of the Shastry-Sutherland Model, [Phys. Rev. Lett. \*\*86\*\*, 520 \(2001\)](#).
  - [9] T. Momoi and K. Totsuka, Magnetization plateaus as insulator-superfluid transitions in quantum spin systems, [Phys. Rev. B \*\*61\*\*, 3231 \(2000\)](#).
  - [10] T. Momoi and K. Totsuka, Magnetization plateaus of the Shastry-Sutherland model for  $\text{SrCu}_2(\text{BO}_3)_2$ : Spin-density wave, supersolid, and bound states, [Phys. Rev. B \*\*62\*\*, 15067 \(2000\)](#).
  - [11] S. Miyahara and K. Ueda, Theory of the orthogonal dimer Heisenberg spin model for  $\text{SrCu}_2(\text{BO}_3)_2$ , [J. Phys.: Condens. Matter \*\*15\*\*, R327 \(2003\)](#).
  - [12] Z. Weihong, C. J. Hamer, and J. Oitmaa, Series expansions for a Heisenberg antiferromagnetic model for  $\text{SrCu}_2(\text{BO}_3)_2$ , [Phys. Rev. B \*\*60\*\*, 6608 \(1999\)](#).
  - [13] C. Knetter, A. Bühler, E. Müller-Hartmann, and G. S. Uhrig, Dispersion and Symmetry of Bound States in the Shastry-Sutherland Model, [Phys. Rev. Lett. \*\*85\*\*, 3958 \(2000\)](#).

- [14] O. Cépas, K. Kakurai, L. P. Regnault, T. Ziman, J. P. Boucher, N. Aso, M. Nishi, H. Kageyama, and Y. Ueda, Dzyaloshinski-Moriya Interaction in the 2D Spin Gap System  $\text{SrCu}_2(\text{BO}_3)_2$ , [Phys. Rev. Lett.](#) **87**, 167205 (2001).
- [15] P. A. McClarty, F. Krüger, T. Guidi, S. F. Parker, K. Refson, A. W. Parker, D. Prabhakaran, and R. Coldea, Topological triplon modes and bound states in a Shastry–Sutherland magnet, [Nat. Phys.](#) **13**, 736 (2017).
